# Supplementary material for: Theme-driven Keyphrase Extraction to Analyze Social Media Discourse
Source: arXiv:2301.11508 source file (2023-05-28)
Supplement: Supplementary file 2 [file supplementary.tex]

% \section{Supplementary}

% \subsection{TKE with ChatGPT Experiments}

% In our study, we conducted a series of experiments to evaluate the performance of different configurations of GPT KE. The experiments were designed with various parameters such as the length and complexity of the prompt, the "temperature" setting of the model, the specificity of the prompt to a particular theme, the number of examples provided to the model, and the randomness of these examples.

% The nomenclature of the runs was designed as follows:
% \begin{itemize}
%     \item basic: Represents a simple, short, zero-shot prompt, like 'extract keyphrases'.
%     \item fancy: Represents a longer and more detailed prompt, which includes our detailed definitions of keyphrases.
%     \item hot: Indicates a temperature setting of 0.95.
%     \item cold: Indicates a temperature setting of 0.1 (all future runs, including all of them used in the final study, were conducted with temperature set to 0.0).
%     \item theme specific in the name: Indicates that the prompt was only for a specific theme.
%     \item combined: Represents the combined results of runs for a single theme.
%     \item fewshot: Represents any run that included multiple examples.
%     \item random: Represents fewshot runs with randomly selected examples.
%     \item 3: Represents any fewshot run with three examples.
%     \item 5: Represents any fewshot run with five examples.
% \end{itemize}

% \subsubsection{Prompts}

% These were all the prompt variations used to run our experiments. 
% prompt_basic = 'Extract a list of important and minimal keyphrases from the following Reddit post:\n{}'

% prompt_fancy = 'Perform keyphrase extraction on the following Reddit post for opioid use disorder (OUD) recovery, aligned with four main themes: "Treatment Options", "Substance Dependency & Recovery", "Medical History", and "Psychophysical Effects". The keyphrases should be relevant to the lived experiences of individuals affected by OUD, and should capture domain-specific terminology while normalizing diverse vocabulary, slang, and misspellings associated with informal discussions online. The keyphrases should be specific and non-ambiguous while balancing the trade-offs between univocity and generalizability. Provide a list of high-quality keyphrases that capture the key aspects of OUD recovery, aligned with the four main themes, and grounded in substance use research. Consider research on substance use, addiction, and recovery, as well as guidance from available resources, including governmental agencies, academic institutions, and public health organizations.\n\nReddit post: \n{}'

% prompt_treatment_options = 'I want you to act as a keyphrase extractor. I will provide a full Reddit post, and your task is to perform keyphrase extraction for opioid use disorder (OUD) recovery, aligned with the theme of "Treatment Options". This category covers keyphrases related to different treatment options used for recovery, including medications used to treat OUD (e.g., Buprenorphine, Methadone, or their formulations), psychotherapy, behavioral counseling, or other medications used to cope with withdrawal or other psychophysical effects (e.g., using melatonin to help with insomnia while in recovery). We consider prescribed medications, over-the-counter medications, herbal supplements, and other therapeutic options as potential candidates for keyphrases. The keyphrases should be relevant to the lived experiences of individuals affected by OUD and grounded in substance use research, while also normalizing diverse vocabulary, slang, and misspellings associated with informal discussions online. The keyphrases should be specific and non-ambiguous while balancing the trade-offs between univocity and generalizability. Provide a list of high-quality keyphrases that capture the key aspects of OUD recovery, aligned with the theme and informed by available resources, including governmental agencies, academic institutions, and public health organizations. The keyphrases should be a minimal representation (select as few as possible), and some posts may not contain any. Format everything as a python list and only output that.\n\nThe Reddit post: \n{}'

% prompt_substance_recovery = 'I want you to act as a keyphrase extractor. I will provide a full Reddit post, and your task is to perform keyphrase extraction for substance dependency and recovery. This category covers keyphrases related to the history of substance use (e.g., "fentanyl"), co-occurring substance use (e.g., "tobacco", "alcohol"), and critical factors in recovery (e.g., recovery, relapse). We consider both prescribed and self-administered substances. The keyphrases should be relevant to the lived experiences of individuals affected by substance dependency and recovery and grounded in substance use research, while also normalizing diverse vocabulary, slang, and misspellings associated with informal discussions online. The keyphrases should be specific and non-ambiguous while balancing the trade-offs between univocity and generalizability. Provide a list of high-quality keyphrases that capture the key aspects of substance dependency and recovery, aligned with the theme and informed by available resources, including governmental agencies, academic institutions, and public health organizations. The keyphrases should be a minimal representation (select as few as possible), and some posts may not contain any. Format everything as a python list and only output that.\n\nThe Reddit post: \n{}'

% prompt_medical_history = 'I want you to act as a keyphrase extractor. I will provide a full Reddit post, and your task is to perform keyphrase extraction for Medical History. This category covers keyphrases concerning medical history, including diagnosis and self-diagnosis of any physical and mental health conditions, relevant medical procedures (e.g., major surgery), or critical family medical history. We consider any relevant medical history beyond substance dependency/recovery. The keyphrases should be relevant to the lived experiences of individuals affected by medical conditions and grounded in medical research, while also normalizing diverse vocabulary, slang, and misspellings associated with informal discussions online. The keyphrases should be specific and non-ambiguous while balancing the trade-offs between univocity and generalizability. Provide a list of high-quality keyphrases that capture the key aspects of medical history, aligned with the theme and informed by available resources, including governmental agencies, academic institutions, and public health organizations. The keyphrases should be a minimal representation (select as few as possible), and some posts may not contain any. Format everything as a python list and only output that. \n\nThe Reddit post: \n{}'

% prompt_psychophysical_effects = 'I want you to act as a keyphrase extractor. I will provide a full Reddit post, and your task is to perform keyphrase extraction for opioid use disorder (OUD) recovery, aligned with the theme of "Psychophysical Effects". This category covers keyphrases regarding any physical or psychological effects and symptoms associated with OUD recovery, e.g., psychological effects relevant to withdrawal, precipitated withdrawal, and side effects of medications. We consider both the subjective and objective experiences of individuals affected by OUD and grounded in substance use research, while also normalizing diverse vocabulary, slang, and misspellings associated with informal discussions online. The keyphrases should be specific and non-ambiguous while balancing the trade-offs between univocity and generalizability. Provide a list of high-quality keyphrases that capture the key aspects of OUD recovery, aligned with the theme and informed by available resources, including governmental agencies, academic institutions, and public health organizations. The keyphrases should be a minimal representation (select as few as possible), and some posts may not contain any. Format everything as a python list and only output that.\n\nThe Reddit post: \n{}'

% prompt_fancy_few_shot_3 = "I want you to act as a keyphrase extractor. Perform keyphrase extraction on the following Reddit post for opioid use disorder (OUD) recovery, aligned with four main themes: \"Treatment Options\", \"Substance Dependency & Recovery\", \"Medical History\", and \"Psychophysical Effects\". The keyphrases should be relevant to the lived experiences of individuals affected by OUD, and should capture domain-specific terminology while normalizing diverse vocabulary, slang, and misspellings associated with informal discussions online. The keyphrases should be specific and non-ambiguous while balancing the trade-offs between univocity and generalizability. Provide a list of high-quality keyphrases that capture the key aspects of OUD recovery, aligned with the four main themes, and grounded in substance use research. Consider research on substance use, addiction, and recovery, as well as guidance from available resources, including governmental agencies, academic institutions, and public health organizations.\n\nExample 1\ntitle: {{getting on suboxone}}\n\nbody: {{\nI just got back from Florida and have been clean from dope for 9 months but the cravings are setting in what is the best way to go about getting on suboxone?? can my PCM prescribe??\n}}\n\nkeyphrases: ['suboxone', 'dope', 'cravings', 'clean']\n\nExample 2\ntitle: {{Been Clean on Subs for 80 days , questions.}}\n\nbody: {{\nHey folks. Background .. years of pain management. Things got out of control. My drug was oxycodone. When I stopped I was taking at least 400Mg a day and up to 600Mg when available. I was on levels that high for at least 8 months. I inducted to subs with minimal issues. I was RX'd 16mg (8mg 2x day). I dose when I get up (around 9:30 AM and again around 3:30 PM). I am not taking what I am RX'd. I am taking 6Mg in the morning and 6Mg in the afternoon. \n\nEverything started off well .. I felt full of energy and even had some sleep problems. Now I am tired all the time. I find it VERY hard to get up in the morning. It seems like I can't get going until about 2 hours after my AM dose. It also seems like my muscles are weak.\n\nI own my own business and can go in whenever I want but my goal is to be able to get up earlier. I am thinking about starting to set an alarm for 6AM to dose with hopes of coming alive to be in the office around 9. \n\nDoes anyone have any suggestions? I still think about having an oxymoron bender here and there and just tell myself how much better things are getting in my life without the pills. I wouldn't say I'm having any bad cravings or dreams. \n\nAny input would be greatly appreciated!\n\nKeep Up the Good Fight!\nK8ight \n}}\n\nkeyphrases: ['subs', 'oxymoron', 'pain management', 'tired', 'sleep', 'muscles', 'oxycodone', 'pills']\n\nExample 3\ntitle: {{Getting a higher dose of Suboxone.}}\n\nbody: {{\nI've been on Suboxone for one year now with the same doctor. I was very quickly able to drop from 16mg per day to 2mg per day. Over the past few months my script has been running out a few days early, but this month my script will be out 10 days short. It's been a horrible 20 days. So many bad and good things have been happening all at once in my life and I am extremely overwhelmed. Due to being overwhelmed, I have taken 3mg a day in order to keep myself from the edge of relapse. I decided I should tell my doctor about this instead of running out early every single month and struggling to make it until that next refill date. Luckily my appointment is early this month so I won't have to deal with going through withdrawals. Do you think my doctor will understand and up my dose? If it matters, I have passed every single drug test and have had a good relationship with this doctor. \n}}\n\nkeyphrases: ['doctor', 'relapse', 'withdrawals', 'script', 'Suboxone']\n\nNow extract keyprases from this Reddit post:\n{}"
% prompt_treatment_options_few_shot_3 = "I want you to act as a keyphrase extractor. I will provide a full Reddit post, and your task is to perform keyphrase extraction for opioid use disorder (OUD) recovery, aligned with the theme of \"Treatment Options\". This category covers keyphrases related to different treatment options used for recovery, including medications used to treat OUD (e.g., Buprenorphine, Methadone, or their formulations), psychotherapy, behavioral counseling, or other medications used to cope with withdrawal or other psychophysical effects (e.g., using melatonin to help with insomnia while in recovery). We consider prescribed medications, over-the-counter medications, herbal supplements, and other therapeutic options as potential candidates for keyphrases. The keyphrases should be relevant to the lived experiences of individuals affected by OUD and grounded in substance use research, while also normalizing diverse vocabulary, slang, and misspellings associated with informal discussions online. The keyphrases should be specific and non-ambiguous while balancing the trade-offs between univocity and generalizability. Provide a list of high-quality keyphrases that capture the key aspects of OUD recovery, aligned with the theme and informed by available resources, including governmental agencies, academic institutions, and public health organizations. The keyphrases should be a minimal representation (select as few as possible), and some posts may not contain any.\n\nExample 1\ntitle: {{getting on suboxone}}\n\nbody: {{\nI just got back from Florida and have been clean from dope for 9 months but the cravings are setting in what is the best way to go about getting on suboxone?? can my PCM prescribe??\n}}\n\nkeyphrases: ['suboxone']\n\nExample 2\ntitle: {{Been Clean on Subs for 80 days , questions.}}\n\nbody: {{\nHey folks. Background .. years of pain management. Things got out of control. My drug was oxycodone. When I stopped I was taking at least 400Mg a day and up to 600Mg when available. I was on levels that high for at least 8 months. I inducted to subs with minimal issues. I was RX'd 16mg (8mg 2x day). I dose when I get up (around 9:30 AM and again around 3:30 PM). I am not taking what I am RX'd. I am taking 6Mg in the morning and 6Mg in the afternoon. \n\nEverything started off well .. I felt full of energy and even had some sleep problems. Now I am tired all the time. I find it VERY hard to get up in the morning. It seems like I can't get going until about 2 hours after my AM dose. It also seems like my muscles are weak.\n\nI own my own business and can go in whenever I want but my goal is to be able to get up earlier. I am thinking about starting to set an alarm for 6AM to dose with hopes of coming alive to be in the office around 9. \n\nDoes anyone have any suggestions? I still think about having an oxymoron bender here and there and just tell myself how much better things are getting in my life without the pills. I wouldn't say I'm having any bad cravings or dreams. \n\nAny input would be greatly appreciated!\n\nKeep Up the Good Fight!\nK8ight \n}}\n\nkeyphrases: ['subs', 'Subs', 'pills']\n\nExample 3\ntitle: {{Getting a higher dose of Suboxone.}}\n\nbody: {{\nI've been on Suboxone for one year now with the same doctor. I was very quickly able to drop from 16mg per day to 2mg per day. Over the past few months my script has been running out a few days early, but this month my script will be out 10 days short. It's been a horrible 20 days. So many bad and good things have been happening all at once in my life and I am extremely overwhelmed. Due to being overwhelmed, I have taken 3mg a day in order to keep myself from the edge of relapse. I decided I should tell my doctor about this instead of running out early every single month and struggling to make it until that next refill date. Luckily my appointment is early this month so I won't have to deal with going through withdrawals. Do you think my doctor will understand and up my dose? If it matters, I have passed every single drug test and have had a good relationship with this doctor. \n}}\n\nkeyphrases: ['script', 'Suboxone']\n\nNow extract keyprases from this Reddit post: \n{}"

% prompt_substance_recovery_few_shot_3 = "I want you to act as a keyphrase extractor. I will provide a full Reddit post, and your task is to perform keyphrase extraction for substance dependency and recovery. This category covers keyphrases related to the history of substance use (e.g., \"fentanyl\"), co-occurring substance use (e.g., \"tobacco\", \"alcohol\"), and critical factors in recovery (e.g., recovery, relapse). We consider both prescribed and self-administered substances. The keyphrases should be relevant to the lived experiences of individuals affected by substance dependency and recovery and grounded in substance use research, while also normalizing diverse vocabulary, slang, and misspellings associated with informal discussions online. The keyphrases should be specific and non-ambiguous while balancing the trade-offs between univocity and generalizability. Provide a list of high-quality keyphrases that capture the key aspects of substance dependency and recovery, aligned with the theme and informed by available resources, including governmental agencies, academic institutions, and public health organizations. The keyphrases should be a minimal representation (select as few as possible), and some posts may not contain any.'\n\nExample 1\ntitle: {{getting on suboxone}}\n\nbody: {{\nI just got back from Florida and have been clean from dope for 9 months but the cravings are setting in what is the best way to go about getting on suboxone?? can my PCM prescribe??\n}}\n\nkeyphrases: ['suboxone', 'dope', 'clean']\n\nExample 2\ntitle: {{Been Clean on Subs for 80 days , questions.}}\n\nbody: {{\nHey folks. Background .. years of pain management. Things got out of control. My drug was oxycodone. When I stopped I was taking at least 400Mg a day and up to 600Mg when available. I was on levels that high for at least 8 months. I inducted to subs with minimal issues. I was RX'd 16mg (8mg 2x day). I dose when I get up (around 9:30 AM and again around 3:30 PM). I am not taking what I am RX'd. I am taking 6Mg in the morning and 6Mg in the afternoon. \n\nEverything started off well .. I felt full of energy and even had some sleep problems. Now I am tired all the time. I find it VERY hard to get up in the morning. It seems like I can't get going until about 2 hours after my AM dose. It also seems like my muscles are weak.\n\nI own my own business and can go in whenever I want but my goal is to be able to get up earlier. I am thinking about starting to set an alarm for 6AM to dose with hopes of coming alive to be in the office around 9. \n\nDoes anyone have any suggestions? I still think about having an oxymoron bender here and there and just tell myself how much better things are getting in my life without the pills. I wouldn't say I'm having any bad cravings or dreams. \n\nAny input would be greatly appreciated!\n\nKeep Up the Good Fight!\nK8ight \n}}\n\nkeyphrases: ['subs', 'pain management', 'oxycodone', 'pills']\n\nExample 3\ntitle: {{Getting a higher dose of Suboxone.}}\n\nbody: {{\nI've been on Suboxone for one year now with the same doctor. I was very quickly able to drop from 16mg per day to 2mg per day. Over the past few months my script has been running out a few days early, but this month my script will be out 10 days short. It's been a horrible 20 days. So many bad and good things have been happening all at once in my life and I am extremely overwhelmed. Due to being overwhelmed, I have taken 3mg a day in order to keep myself from the edge of relapse. I decided I should tell my doctor about this instead of running out early every single month and struggling to make it until that next refill date. Luckily my appointment is early this month so I won't have to deal with going through withdrawals. Do you think my doctor will understand and up my dose? If it matters, I have passed every single drug test and have had a good relationship with this doctor. \n}}\n\nkeyphrases: ['relapse', 'script', 'Suboxone']\n\nNow extract keyprases from this Reddit post: \n{}"

% prompt_medical_history_few_shot_3 = "I want you to act as a keyphrase extractor. I will provide a full Reddit post, and your task is to perform keyphrase extraction for Medical History. This category covers keyphrases concerning medical history, including diagnosis and self-diagnosis of any physical and mental health conditions, relevant medical procedures (e.g., major surgery), or critical family medical history. We consider any relevant medical history beyond substance dependency/recovery. The keyphrases should be relevant to the lived experiences of individuals affected by medical conditions and grounded in medical research, while also normalizing diverse vocabulary, slang, and misspellings associated with informal discussions online. The keyphrases should be specific and non-ambiguous while balancing the trade-offs between univocity and generalizability. Provide a list of high-quality keyphrases that capture the key aspects of medical history, aligned with the theme and informed by available resources, including governmental agencies, academic institutions, and public health organizations. The keyphrases should be a minimal representation (select as few as possible), and some posts may not contain any.\n\nExample 1\ntitle: {{getting on suboxone}}\n\nbody: {{\nI just got back from Florida and have been clean from dope for 9 months but the cravings are setting in what is the best way to go about getting on suboxone?? can my PCM prescribe??\n}}\n\nkeyphrases: ['clean']\n\nExample 2\ntitle: {{Been Clean on Subs for 80 days , questions.}}\n\nbody: {{\nHey folks. Background .. years of pain management. Things got out of control. My drug was oxycodone. When I stopped I was taking at least 400Mg a day and up to 600Mg when available. I was on levels that high for at least 8 months. I inducted to subs with minimal issues. I was RX'd 16mg (8mg 2x day). I dose when I get up (around 9:30 AM and again around 3:30 PM). I am not taking what I am RX'd. I am taking 6Mg in the morning and 6Mg in the afternoon. \n\nEverything started off well .. I felt full of energy and even had some sleep problems. Now I am tired all the time. I find it VERY hard to get up in the morning. It seems like I can't get going until about 2 hours after my AM dose. It also seems like my muscles are weak.\n\nI own my own business and can go in whenever I want but my goal is to be able to get up earlier. I am thinking about starting to set an alarm for 6AM to dose with hopes of coming alive to be in the office around 9. \n\nDoes anyone have any suggestions? I still think about having an oxymoron bender here and there and just tell myself how much better things are getting in my life without the pills. I wouldn't say I'm having any bad cravings or dreams. \n\nAny input would be greatly appreciated!\n\nKeep Up the Good Fight!\nK8ight \n}}\n\nkeyphrases: ['pain management']\n\nExample 3\ntitle: {{Getting a higher dose of Suboxone.}}\n\nbody: {{\nI've been on Suboxone for one year now with the same doctor. I was very quickly able to drop from 16mg per day to 2mg per day. Over the past few months my script has been running out a few days early, but this month my script will be out 10 days short. It's been a horrible 20 days. So many bad and good things have been happening all at once in my life and I am extremely overwhelmed. Due to being overwhelmed, I have taken 3mg a day in order to keep myself from the edge of relapse. I decided I should tell my doctor about this instead of running out early every single month and struggling to make it until that next refill date. Luckily my appointment is early this month so I won't have to deal with going through withdrawals. Do you think my doctor will understand and up my dose? If it matters, I have passed every single drug test and have had a good relationship with this doctor. \n}}\n\nkeyphrases: ['relapse', 'withdrawals']\n\nNow extract keyprases from this Reddit post: \n{}"

% prompt_psychophysical_effects_few_shot_3 = "I want you to act as a keyphrase extractor. I will provide a full Reddit post, and your task is to perform keyphrase extraction for opioid use disorder (OUD) recovery, aligned with the theme of \"Psychophysical Effects\". This category covers keyphrases regarding any physical or psychological effects and symptoms associated with OUD recovery, e.g., psychological effects relevant to withdrawal, precipitated withdrawal, and side effects of medications. We consider both the subjective and objective experiences of individuals affected by OUD and grounded in substance use research, while also normalizing diverse vocabulary, slang, and misspellings associated with informal discussions online. The keyphrases should be specific and non-ambiguous while balancing the trade-offs between univocity and generalizability. Provide a list of high-quality keyphrases that capture the key aspects of OUD recovery, aligned with the theme and informed by available resources, including governmental agencies, academic institutions, and public health organizations. The keyphrases should be a minimal representation (select as few as possible), and some posts may not contain any.\n\nExample 1\ntitle: {{getting on suboxone}}\n\nbody: {{\nI just got back from Florida and have been clean from dope for 9 months but the cravings are setting in what is the best way to go about getting on suboxone?? can my PCM prescribe??\n}}\n\nkeyphrases: ['cravings']\n\nExample 2\ntitle: {{Been Clean on Subs for 80 days , questions.}}\n\nbody: {{\nHey folks. Background .. years of pain management. Things got out of control. My drug was oxycodone. When I stopped I was taking at least 400Mg a day and up to 600Mg when available. I was on levels that high for at least 8 months. I inducted to subs with minimal issues. I was RX'd 16mg (8mg 2x day). I dose when I get up (around 9:30 AM and again around 3:30 PM). I am not taking what I am RX'd. I am taking 6Mg in the morning and 6Mg in the afternoon. \n\nEverything started off well .. I felt full of energy and even had some sleep problems. Now I am tired all the time. I find it VERY hard to get up in the morning. It seems like I can't get going until about 2 hours after my AM dose. It also seems like my muscles are weak.\n\nI own my own business and can go in whenever I want but my goal is to be able to get up earlier. I am thinking about starting to set an alarm for 6AM to dose with hopes of coming alive to be in the office around 9. \n\nDoes anyone have any suggestions? I still think about having an oxymoron bender here and there and just tell myself how much better things are getting in my life without the pills. I wouldn't say I'm having any bad cravings or dreams. \n\nAny input would be greatly appreciated!\n\nKeep Up the Good Fight!\nK8ight \n}}\n\nkeyphrases: ['tired', 'sleep']\n\nExample 3\ntitle: {{Getting a higher dose of Suboxone.}}\n\nbody: {{\nI've been on Suboxone for one year now with the same doctor. I was very quickly able to drop from 16mg per day to 2mg per day. Over the past few months my script has been running out a few days early, but this month my script will be out 10 days short. It's been a horrible 20 days. So many bad and good things have been happening all at once in my life and I am extremely overwhelmed. Due to being overwhelmed, I have taken 3mg a day in order to keep myself from the edge of relapse. I decided I should tell my doctor about this instead of running out early every single month and struggling to make it until that next refill date. Luckily my appointment is early this month so I won't have to deal with going through withdrawals. Do you think my doctor will understand and up my dose? If it matters, I have passed every single drug test and have had a good relationship with this doctor. \n}}\n\nkeyphrases: ['withdrawals']\n\nNow extract keyprases from this Reddit post: \n{}"

% prompt_fancy_few_shot_5 = "Perform keyphrase extraction on the following Reddit post for opioid use disorder (OUD) recovery, aligned with four main themes: \"Treatment Options\", \"Substance Dependency & Recovery\", \"Medical History\", and \"Psychophysical Effects\". The keyphrases should be relevant to the lived experiences of individuals affected by OUD, and should capture domain-specific terminology while normalizing diverse vocabulary, slang, and misspellings associated with informal discussions online. The keyphrases should be specific and non-ambiguous while balancing the trade-offs between univocity and generalizability. Provide a list of high-quality keyphrases that capture the key aspects of OUD recovery, aligned with the four main themes, and grounded in substance use research. Consider research on substance use, addiction, and recovery, as well as guidance from available resources, including governmental agencies, academic institutions, and public health organizations.\n\nExample 1\ntitle: {{getting on suboxone}}\nbody: {{\nI just got back from Florida and have been clean from dope for 9 months but the cravings are setting in what is the best way to go about getting on suboxone?? can my PCM prescribe??\n}}\nkeyphrases: ['suboxone', 'dope', 'cravings', 'clean']\n\nExample 2\ntitle: {{Been Clean on Subs for 80 days , questions.}}\nbody: {{\nHey folks. Background .. years of pain management. Things got out of control. My drug was oxycodone. When I stopped I was taking at least 400Mg a day and up to 600Mg when available. I was on levels that high for at least 8 months. I inducted to subs with minimal issues. I was RX'd 16mg (8mg 2x day). I dose when I get up (around 9:30 AM and again around 3:30 PM). I am not taking what I am RX'd. I am taking 6Mg in the morning and 6Mg in the afternoon.\n\nEverything started off well .. I felt full of energy and even had some sleep problems. Now I am tired all the time. I find it VERY hard to get up in the morning. It seems like I can't get going until about 2 hours after my AM dose. It also seems like my muscles are weak.\n\nI own my own business and can go in whenever I want but my goal is to be able to get up earlier. I am thinking about starting to set an alarm for 6AM to dose with hopes of coming alive to be in the office around 9.\n\nDoes anyone have any suggestions? I still think about having an oxymoron bender here and there and just tell myself how much better things are getting in my life without the pills. I wouldn't say I'm having any bad cravings or dreams.\n\nAny input would be greatly appreciated!\n\nKeep Up the Good Fight!\nK8ight\n}}\nkeyphrases: ['subs', 'oxymoron', 'Subs', 'pain management', 'tired', 'sleep', 'muscles', 'oxycodone', 'pills']\n\nExample 3\ntitle: {{Getting a higher dose of Suboxone.}}\nbody: {{\nI've been on Suboxone for one year now with the same doctor. I was very quickly able to drop from 16mg per day to 2mg per day. Over the past few months my script has been running out a few days early, but this month my script will be out 10 days short. It's been a horrible 20 days. So many bad and good things have been happening all at once in my life and I am extremely overwhelmed. Due to being overwhelmed, I have taken 3mg a day in order to keep myself from the edge of relapse. I decided I should tell my doctor about this instead of running out early every single month and struggling to make it until that next refill date. Luckily my appointment is early this month so I won't have to deal with going through withdrawals. Do you think my doctor will understand and up my dose? If it matters, I have passed every single drug test and have had a good relationship with this doctor.\n}}\nkeyphrases: ['doctor', 'relapse', 'withdrawals', 'script', 'Suboxone']\n\nExample 4\ntitle: {{Thinking of starting on Subs - Some questions.}}\nbody: {{\nSo I'm thinking subs might be useful for me, but I have some questions.\n\nMy first is when should I take my first one? I take poppy pods which last a real long time. If I take a large dose I only start feeling  withdrawals after 48 hours, and even then it's mild. It starts building from there and I can imagine they would get pretty severe at 72 hours (I haven't made it that far in a while). So does 72 hours sound good? Too early/too late?\n\nMy second is what is the shortest time that would be useful? I want to use it strictly to detox, I'm not interested in maintenance. I've heard some people say 7 day detox is best, some say 14, some say 8 week. In your experience what is the best way to use subutex to help detox?\n\nLastly if anyone here is from the UK and wouldn't mind me asking them some questions please let me know!\n\nI have many more questions but that will do for now. Thank you in advance.\n}}\nkeyphrases: ['subs', 'withdrawals', 'detox', 'Subs', 'poppy pods', 'subutex']\n\nExample 5\ntitle: {{dosing question}}\nbody: {{\nIve been on about 12 mg for 5 yrs, some days if im just laying around i dont take my dose for that day. does anyone else do the same thing? i just recently got  script,  been buying off the st for this entire time, maybe its the i dont wanna run out minset trying to save what i can for when i really need it. any info is appreciated. thanks \n}}\nkeyphrases: ['dosing']"

% prompt_fancy_few_shot_10 = "Perform keyphrase extraction on the following Reddit post for opioid use disorder (OUD) recovery, aligned with four main themes: \"Treatment Options\", \"Substance Dependency & Recovery\", \"Medical History\", and \"Psychophysical Effects\". The keyphrases should be relevant to the lived experiences of individuals affected by OUD, and should capture domain-specific terminology while normalizing diverse vocabulary, slang, and misspellings associated with informal discussions online. The keyphrases should be specific and non-ambiguous while balancing the trade-offs between univocity and generalizability. Provide a list of high-quality keyphrases that capture the key aspects of OUD recovery, aligned with the four main themes, and grounded in substance use research. Consider research on substance use, addiction, and recovery, as well as guidance from available resources, including governmental agencies, academic institutions, and public health organizations.\n\nExample 1\ntitle: {{getting on suboxone}}\nbody: {{\nI just got back from Florida and have been clean from dope for 9 months but the cravings are setting in what is the best way to go about getting on suboxone?? can my PCM prescribe??\n}}\nkeyphrases: ['suboxone', 'dope', 'cravings', 'clean']\n\nExample 2\ntitle: {{Been Clean on Subs for 80 days , questions.}}\nbody: {{\nHey folks. Background .. years of pain management. Things got out of control. My drug was oxycodone. When I stopped I was taking at least 400Mg a day and up to 600Mg when available. I was on levels that high for at least 8 months. I inducted to subs with minimal issues. I was RX'd 16mg (8mg 2x day). I dose when I get up (around 9:30 AM and again around 3:30 PM). I am not taking what I am RX'd. I am taking 6Mg in the morning and 6Mg in the afternoon.\n\nEverything started off well .. I felt full of energy and even had some sleep problems. Now I am tired all the time. I find it VERY hard to get up in the morning. It seems like I can't get going until about 2 hours after my AM dose. It also seems like my muscles are weak.\n\nI own my own business and can go in whenever I want but my goal is to be able to get up earlier. I am thinking about starting to set an alarm for 6AM to dose with hopes of coming alive to be in the office around 9.\n\nDoes anyone have any suggestions? I still think about having an oxymoron bender here and there and just tell myself how much better things are getting in my life without the pills. I wouldn't say I'm having any bad cravings or dreams.\n\nAny input would be greatly appreciated!\n\nKeep Up the Good Fight!\nK8ight\n}}\nkeyphrases: ['subs', 'oxymoron', 'Subs', 'pain management', 'tired', 'sleep', 'muscles', 'oxycodone', 'pills']\n\nExample 3\ntitle: {{Getting a higher dose of Suboxone.}}\nbody: {{\nI've been on Suboxone for one year now with the same doctor. I was very quickly able to drop from 16mg per day to 2mg per day. Over the past few months my script has been running out a few days early, but this month my script will be out 10 days short. It's been a horrible 20 days. So many bad and good things have been happening all at once in my life and I am extremely overwhelmed. Due to being overwhelmed, I have taken 3mg a day in order to keep myself from the edge of relapse. I decided I should tell my doctor about this instead of running out early every single month and struggling to make it until that next refill date. Luckily my appointment is early this month so I won't have to deal with going through withdrawals. Do you think my doctor will understand and up my dose? If it matters, I have passed every single drug test and have had a good relationship with this doctor.\n}}\nkeyphrases: ['doctor', 'relapse', 'withdrawals', 'script', 'Suboxone']\n\nExample 4\ntitle: {{Thinking of starting on Subs - Some questions.}}\nbody: {{\nSo I'm thinking subs might be useful for me, but I have some questions.\n\nMy first is when should I take my first one? I take poppy pods which last a real long time. If I take a large dose I only start feeling  withdrawals after 48 hours, and even then it's mild. It starts building from there and I can imagine they would get pretty severe at 72 hours (I haven't made it that far in a while). So does 72 hours sound good? Too early/too late?\n\nMy second is what is the shortest time that would be useful? I want to use it strictly to detox, I'm not interested in maintenance. I've heard some people say 7 day detox is best, some say 14, some say 8 week. In your experience what is the best way to use subutex to help detox?\n\nLastly if anyone here is from the UK and wouldn't mind me asking them some questions please let me know!\n\nI have many more questions but that will do for now. Thank you in advance.\n}}\nkeyphrases: ['subs', 'withdrawals', 'detox', 'Subs', 'poppy pods', 'subutex']\n\nExample 5\ntitle: {{dosing question}}\nbody: {{\nIve been on about 12 mg for 5 yrs, some days if im just laying around i dont take my dose for that day. does anyone else do the same thing? i just recently got  script,  been buying off the st for this entire time, maybe its the i dont wanna run out minset trying to save what i can for when i really need it. any info is appreciated. thanks \n}}\nkeyphrases: ['dosing']\n\nExample 6\ntitle: {{Switching from methadone to subs}}\nbody: {{\nSo my last dose was Thursday at 60mg.. I went down 10mg every 4 days from 130.\nFor reasons beyond my control I didn't get to titrate down to 30 as planned before leaving the clinic. Luckily, the doctor at the Suboxone clinic saw me early (yesterday) and wrote my script as long as I promised to wait until I was in full blown withdrawal before taking anything. She wrote me a weeks worth of Subutex, 21 8mg tablets and then next Friday I go see her and get my Suboxone script. She explained that the transition would be a bit smoother with just bupe instead of the bupe w/ naloxone. Anyway, I understand how it all works and why I should wait. I am going to wait as long as I can because I am terrified of pwd. I was just hoping there might be someone here who has also made the switch from methadone to bupe and could give me some advice. Thanks\n}}\nkeyphrases: ['bupe', 'pwd', 'methadone', 'Switching', 'Suboxone', 'switch', 'Subutex', 'subs', 'terrified', 'naloxone']\n\nExample 7\ntitle: {{I need some help with dosing}}\nbody: {{\nA little backstory: I have extreme chronic pain, and where I live pain medicine is controlled and so there are no doctors who will prescribe me anything for pain, which is frustrating.\nAnyway, I found a guy who has been selling me percocets for the last 6 months and I have been taking about 6 a day, sometimes more depending on how bad my pain is. The guy who provided them doesn't have anymore at the moment and I am suffering from withdrawals. The guy gave me Suboxone and said it helps with withdrawals, but the thing is he said he has no idea how much or how often I should take them and because this is the first time I have heard of this stuff, I'm kind of afraid of taking them especially since I don't know how much to take or how often to take them. \n\nSo my questions are, what's the starting dose of this stuff? How often should I take them? How do I ingest it, do I swallow them? I thought I read somewhere you put them under your tongue, is this true? He gave me 2mg and 8 mg pills. Is that too much or too little? How long after my last percocet dose should I take it? My last percocet dose was 18 hours ago and I feel awful, and it will only get worse, right?  \nI'm so torn on what to do. On one hand I want this crappy feeling to go away now, but on the other hand I'm too afraid to take something foreign to me that has never been prescribed. \n\nNot only do I have lots of questions about Suboxone, but I'm also looking for support. I'm just really scared right now because I feel like I'm dying. \n}}\nkeyphrases: ['feel awful', 'doctors', 'pain medicine', 'chronic pain', 'percocets', 'withdrawals', 'Suboxone', 'percocet', 'dose']\n\nExample 8\ntitle: {{Subs affecting my BM (very personal)}}\nbody: {{\nSorry for the kinda gross topic but everybody poops and then when you canâ€™t itâ€™s a freaking problem. \nIâ€™m on 4mg of subs a day and had been constipated for over a week. I took miralax for 3 days, then when nothing happened took a stimulant laxative, nothing happened for 2 whole days, then finally drank milk of magnesia last night and now Iâ€™m literally peeing out of my asshole.  How the fuck can I have a regular bowel movement.??????\nAnd yes Iâ€™m drinking a crap ton of water, and including fiber in my diet everyday and exercising. \n}}\nkeyphrases: ['milk of magnesia', 'BM', 'miralax', 'stimulant laxative', 'constipated', 'Subs', 'subs']\n\nExample 9\ntitle: {{How do you treat your Constipation?}}\nbody: {{\nSubs make me constipated and itâ€™s becoming a pain in my ass. I wanna poop like normal folk poop! How does yâ€™all deal with this side effect?\n}}\nkeyphrases: ['Subs', 'constipated', 'Constipation']\n\nExample 10\ntitle: {{Jumped to 0 today}}\nbody: {{\nI have been on subs for over 5 years, not prescribed but a connect who is. I have quit once before but I stopped using all drugs last time for about 2 months (for a job). \n\nMan am I feeling horrible today. I jumped from about a 0.0625 mg which is pretty much nothing. I have been taking cbd and its been helping me sleep, I also have some kratom in the back pocket just in case. But I donâ€™t know if I want to use it. \n\nAny thoughts/ideas would be greatly appreciated. \n}}\nkeyphrases: ['cbd', 'subs', 'kratom', 'feeling horrible']"

% prompt_basic_few_shot_template = "Extract a list of the most important and minimal keyphrases."

% prompt_fancy_few_shot_template = "I want you to act as a keyphrase extractor. Perform keyphrase extraction on the following Reddit post for opioid use disorder (OUD) recovery, aligned with four main themes: \"Treatment Options\", \"Substance Dependency & Recovery\", \"Medical History\", and \"Psychophysical Effects\". The keyphrases should be relevant to the lived experiences of individuals affected by OUD, and should capture domain-specific terminology while normalizing diverse vocabulary, slang, and misspellings associated with informal discussions online. The keyphrases should be specific and non-ambiguous while balancing the trade-offs between univocity and generalizability. Provide a list of high-quality keyphrases that capture the key aspects of OUD recovery, aligned with the four main themes, and grounded in substance use research. Consider research on substance use, addiction, and recovery, as well as guidance from available resources, including governmental agencies, academic institutions, and public health organizations."

% By systematically varying these parameters and using a diverse set of evaluation metrics, we aim to provide a comprehensive understanding of how the GPT KE model performs under various conditions.
    

% \subsection{Normalization}

% This section briefly describes our normalization process. Following are the steps that we followed to normalize the keyphrases.
% \subsubsection{Identification of ``Other" keyphrases}
% Some keyphrases may be important to the post but were not in line with our research questions. Singleton verbs, adjectives, or modifiers all fall into this category. Examples include, \textit{adjust}, \textit{expect},  \textit{acute},  \textit{accidentally}, \textit{expensive}, etc. We used manual inspection to identify such keyphrases. These keyphrases were added to the ``Other" category. 

% \subsubsection{Mapping unigram keyphrases with common stems}
% We additionally perform stemming of keyphrases. All unigrams in our dataset that shared a common stem pattern were mapped to that single variation. For example, \textit{craving} and \textit{cravings} were generated from the stem \textit{crave}, whereas \textit{detox} is the stem for both \textit{detoxing} and \textit{detoxification}. 
% % We used the PorterStemmer python package (version 0.5) to determine the stems. 

% \subsubsection{Mapping semantically similar keyphrases}
% An essential normalization step was to map all keyphrases with the same meaning. The shorthand of keyphrases (\textit{pwd} for \textit{precipitated withdrawal}, \textit{dr} for \textit{doctor}) and misspelled keyphrases (\textit{depressssssed} instead of \textit{depressed}) fall into this category. Since slang and misspellings can arise in numerous variations, we perform the semantic mapping manually. Included in this category are keyphrases consisting of more than one word. Some constituent words can dominate this type of keyphrase (e.g., \textit{online clinic} is dominated by \textit{clinic}). Also, they may possess a different meaning than each of their constituent words (e.g., \textit{precipitated withdrawal} has a different meaning than \textit{precipitated} and \textit{withdrawal}). Thus proper mapping of such keyphrases was identified after careful manual inspection. Finally, keyphrases with similar meanings (e.g., \textit{vomiting} and \textit{puking}) were also mapped in this step using human judgment. It is worth mentioning that we tried to select the generic keyphrases as the representative ones while mapping. For instance, the specific drug \textit{clonazepam} was assigned to the generic group \textit{benzodiazepines} whereas the specialist sub-category of doctor \textit{endocrinologist} was mapped to the more general group \textit{doctor}. However, we did not map some of the specific keyphrases (e.g., \textit{suboxone}, \textit{sublocade}) to their generic group due to their frequent occurrences in the posts. Multiple annotators reviewed all the manual tasks to avoid the potential subjective bias of manual inspections. Each conflicting case was resolved based on majority voting. Finally, an expert reviewed the whole normalization output list and confirmed the validity of the process. Each normalized keyphrase is assigned to predefined categories after a manual review of the keyphrase's context in a sample of posts. 
 
